# Supplementary material for: Deep Hybrid Real and Synthetic Training for Intrinsic Decomposition
Source: arXiv:1807.11226 source file (2018-07-30)
Supplement: Supplementary file 1 [file Appendix.tex]

\section{Appendix}
